# Supplementary material for: Experimental quantum verification in the presence of temporally correlated noise
Source: arXiv:1706.03787 source file (2017-10-04)
Supplement: Supplementary file 1 [file Supplemental_information.pdf]

# Supplemental Information for:
# Experimental quantum verification in the presence of temporally correlated noise

S. Mavadia,[1,2] C. L. Edmunds,[1,2] C. Hempel,[1,2] H. Ball,[1] F. Roy,[1] T. M. Stace,[3] and M. J. Biercuk[†1,2]

[1]*ARC Centre for Engineered Quantum Systems, School of Physics, The University of Sydney, NSW Australia*
[2]*National Measurement Institute, West Lindfield NSW 2070 Australia*
[3]*ARC Centre for Engineered Quantum Systems, School of Physics and Mathematics, The University of Queensland, St Lucia, QLD Australia*
(Dated: Saturday 23rd September, 2017 at 12:28)

## I. Qubit projection estimation

We would like to optimally use the information we collect from the ion to determine the projected state of the qubit after each repetition of an experiment. To do this we implement a Markov model initially published for $^{171}\mathrm{Yb}^+$ in ref. [1]. For the RB experiments described in the main text we combine this information over $r$ repetitions to calculate the most likely projection of the Bloch vector on the $z$-axis. This methodology has a reduced measurement error compared to a simple threshold detection technique based on assigning a state based on whether detected photon counts are above or below a certain threshold.

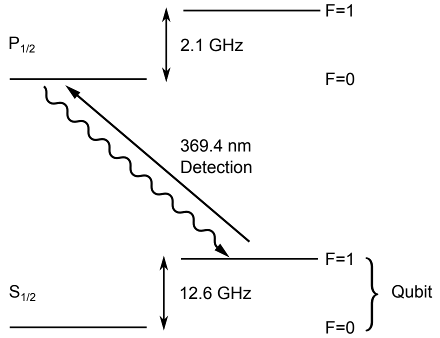


FIG. 1. Relevant energy levels for $^{171}\mathrm{Yb}^+$ and their energy splittings, with the hyperfine structure omitted. The qubit is encoded in the $\mathrm{S}_{1/2}, F = 0, m_F = 0$ and $\mathrm{S}_{1/2}, F = 1, m_F = 0$ states separated by a magnetic dipole transition at 12.64 GHz.

To detect the state of the ion at the end of a sequence of microwave-driven rotations we apply light at 369.4 nm resonant with the optical dipole transition between the $\mathsf{S}_{1/2}, F = 1$ and $\mathsf{P}_{1/2}, F = 0$ states (Fig. 1). During this detection period, an avalanche photodiode registers photons that are scattered if the qubit was projected into the $|F = 1, m_F = 0\rangle$ state, hence denoted "bright state", and no photons if the qubit was projected into the $|F = 0, m_F = 0\rangle$ state.

Due to the proximity of the other electronic levels in the S and P manifolds, off-resonant excitations (proportional to the applied laser power) can occur and change the state of the qubit during the detection period, adversely affecting the detection fidelity. The rate at which these changes occur can be expressed in terms of a bright (dark) state lifetime $\tau_{\mathrm{B}}$ ($\tau_{\mathrm{D}}$).

Rather than simply considering a single transition between the bright and dark states (or visa versa) we can generalise this to multiple transitions within a single measurement detection period [1]. To identify these individual transitions we split the photon deteetion time into equal length sub-bins and make the assumption that there is at most one transition between bright and dark state per sub-bin. We then use the number of photons within each sub-bin and the distribution of photons across sub-bins within a single detection period to determine the likelihood of whether the ion was initially in the bright state or the dark state. For full details of this procedure and a mathematical derivation, see [1].

In our case we employed a detection time of 800 µs which was split into 5 equal length sub-bins of 160 µs. In an ideal case we would use sub-bins which are as short as possible to minimise the likelihood of multiple transitions between dark and bright states in a single sub-bin. In each experimental repetition we calculate the mean detected photon rate in the bright state, $R_B$, and the dark state, $R_D$, by fitting a double Poisson function to a histogram of the entire data set. Typical values are $R_D \approx 0.5\,\mathrm{kHz}$ (resulting from laser scatter and detector dark counts) and $R_B \approx 40\,\mathrm{kHz}$.

The decay rates $\tau_{\mathrm{B,D}}^{-1}$ are measured from separate calibration data where we initialise the ion in either the bright or dark state and then observe the average photon count rate over many repetitions as a function of time. From this information we can calculate the decay rates to be $\tau_B^{-1} \sim 264\,\mathrm{Hz}$ and $\tau_D^{-1} \sim 20\,\mathrm{Hz}$ [1].

In addition to analysing photons in the detection period using sub-bins, we also remove experimental repetitions which do not emit a certain number of photons during the laser cooling period. This accounts for the rare occurrences where the ion is subject

to a collision or other heating effect which may affect the efficacy of experiment.

This procedure is carried out for both RB and GST experiments. However, from this point on, the data area treated differently between the two classes of experiments. For GST experiments we take the most likely outcome for each single repetition, either bright or dark at the beginning of the detection period, and use these outcomes to produce a dataset for input into the pyGSTi software package. For each sequence in the RB experiments, by contrast, we calculate the most likely projection along the z-axis, called survival probability. To do this we implement a Bayesian approach to find the most likely probability distribution of projection onto the $z$-axis, $\phi$. The distribution is discretised, in this case into steps of $10^{-3}$ and and initialised such that the likelihood of measuring a projection along the $z$-axis anywhere between 0 and 1 is equal,

$$\Pr(\phi) = 1/K, \tag{1}$$

where $K$ is a normalisation term. We then condition this probability on the observed photon distribution, $p_\varphi$ such that

$$\Pr(\phi|p_\varphi) = K^{-1}\prod \Pr(p_\varphi|\phi). \tag{2}$$

Where $\Pr(p_\varphi|\phi)$ is calculated from the likelihood of finding the qubit in either the $|1\rangle$ or $|0\rangle$ state,

$$\Pr(p_\varphi|\phi) = \Pr(p_\varphi||1\rangle)\Pr(|1\rangle|\phi) + \Pr(p_\varphi||0\rangle)\Pr(|0\rangle|\phi). \tag{3}$$

The terms $\Pr(p_\varphi||1\rangle)$ and $\Pr(p_\varphi||0\rangle)$ are the likelihoods of measuring $p_\varphi$ photon distribution given that we start in the bright or dark state respectively and are calculated via the Markov model described above. The values $\Pr(|1\rangle|\phi)$ and $\Pr(|0\rangle|\phi)$ are the probabilities of projecting the qubit into either the $|1\rangle$ or $|0\rangle$ state, during detection, given a particular state $\phi$. We incrementally update $\Pr(\phi|p_\varphi)$ by adding information for each repetition across all of the noise realisations. To find the most likely outcome for a particular sequence we then calculate the mean of this distribution.

## II. Unitary rotations in the presence of concurrent $\hat{\sigma}_z$ noise

Here we provide the specific matrix form of the unitary operations employed in GST experiments and simulations where the error model involves a concurrently applied (as opposed to post-multiplied) $\hat{\sigma}_z$ Hamiltonian term. The deliberately introduced $\hat{\sigma}_z$ errors are implemented via a fixed detuning $\Delta$ from qubit's transition frequency. The unperturbed Clifford operations are given by

$$\hat{C}_{\mathbb{1}}(\theta) = e^{-i\frac{\theta}{2}\hat{\sigma}_{\mathbb{1}}}, \tag{4}$$
$$\hat{C}_x(\theta) = e^{-i\frac{\theta}{2}\hat{\sigma}_x}, \tag{5}$$
$$\hat{C}_y(\theta) = e^{-i\frac{\theta}{2}\hat{\sigma}_y}, \tag{6}$$
$$\hat{C}_z(\theta) = e^{-i\frac{\theta}{2}\hat{\sigma}_z}, \tag{7}$$

where rotation angle $\theta \in \{-\pi/2, \pi/2, \pi\}$. In the presence of engineered $\hat{\sigma}_z$ errors, the effective error magnitude relative to the $\Omega$ the Rabi frequency, $\delta = \Delta/\Omega$, modifies the unitary evolution of our gates by introducing concurrent $\hat{\sigma}_z$ rotation:

$$\tilde{C}_{\mathbb{1}}(\theta) = e^{-i\left(\frac{\theta}{2}\hat{\sigma}_{\mathbb{1}} + \frac{|\theta|}{2}\delta\hat{\sigma}_z\right)}, \tag{8}$$
$$\tilde{C}_x(\theta) = e^{-i\left(\frac{\theta}{2}\hat{\sigma}_x + \frac{|\theta|}{2}\delta\hat{\sigma}_z\right)}, \tag{9}$$
$$\tilde{C}_y(\theta) = e^{-i\left(\frac{\theta}{2}\hat{\sigma}_y + \frac{|\theta|}{2}\delta\hat{\sigma}_z\right)}, \tag{10}$$
$$\tilde{C}_z(\theta) = e^{-i\frac{\theta}{2}\hat{\sigma}_z}, \tag{11}$$

yielding the modified gate unitaries

$$\tilde{C}_x(\theta,\Delta,\Omega)=\begin{pmatrix}\cos\left(\frac{\theta\sqrt{\Delta^2+\Omega^2}}{2\Omega}\right)-\frac{i\Delta|\theta|\sin\left(\frac{\sqrt{\theta^2(\Delta^2+\Omega^2)}}{2\Omega}\right)}{\sqrt{\theta^2(\Delta^2+\Omega^2)}} & -\frac{i\Omega\sin\left(\frac{\theta\sqrt{\Delta^2+\Omega^2}}{2\Omega}\right)}{\sqrt{\Delta^2+\Omega^2}}\\ -\frac{i\Omega\sin\left(\frac{\theta\sqrt{\Delta^2+\Omega^2}}{2\Omega}\right)}{\sqrt{\Delta^2+\Omega^2}} & \cos\left(\frac{\theta\sqrt{\Delta^2+\Omega^2}}{2\Omega}\right)+\frac{i\Delta|\theta|\sin\left(\frac{\sqrt{\theta^2(\Delta^2+\Omega^2)}}{2\Omega}\right)}{\sqrt{\theta^2(\Delta^2+\Omega^2)}}\end{pmatrix},$$

$$\tilde{C}_y(\theta,\Delta,\Omega)=\begin{pmatrix}\cosh\left(\frac{\sqrt{-\theta^2(\Delta^2+\Omega^2)}}{2\Omega}\right)-\frac{i\Delta|\theta|\sinh\left(\frac{\sqrt{-\theta^2(\Delta^2+\Omega^2)}}{2\Omega}\right)}{\sqrt{-\theta^2(\Delta^2+\Omega^2)}} & -\frac{\theta\Omega\sinh\left(\frac{\sqrt{-\theta^2(\Delta^2+\Omega^2)}}{2\Omega}\right)}{\sqrt{-\theta^2(\Delta^2+\Omega^2)}}\\ \frac{\theta\Omega\sinh\left(\frac{\sqrt{-\theta^2(\Delta^2+\Omega^2)}}{2\Omega}\right)}{\sqrt{-\theta^2(\Delta^2+\Omega^2)}} & \cosh\left(\frac{\sqrt{-\theta^2(\Delta^2+\Omega^2)}}{2\Omega}\right)+\frac{i\Delta|\theta|\sinh\left(\frac{\sqrt{-\theta^2(\Delta^2+\Omega^2)}}{2\Omega}\right)}{\sqrt{-\theta^2(\Delta^2+\Omega^2)}}\end{pmatrix},$$

$$\tilde{C}_{\mathbb{I}}(\theta,\Delta,\Omega)=\begin{pmatrix}e^{-\frac{i(\theta\Omega+\Delta|\theta|)}{2\Omega}} & 0\\ 0 & e^{\frac{i(\Delta|\theta|-\theta\Omega)}{2\Omega}}\end{pmatrix}.$$

Note that $\tilde{C}_z=\hat{C}_z$ because rotations around the $z$-axis are carried out instantaneously by changing the phase of the microwave synthesizer employed in our experiments (referred to as a "VSG").

## III. Experimental noise engineering

The detunings $\Delta$ used to engineer slowly or rapidly-varying noise are derived from sampling a Gaussian noise distribution $N(0,\sigma^2)$ of a specified root-mean-square width $\sigma$. For each $\Delta_n$ of the $N=200$ noise realisations, the noise distribution gets sampled either once (slowly-varying) or $J$ times, for a sequence of length $J$ gates (rapidly-varying). Error accumulates, as illustrated in Fig. 2, during the gate's nonzero duration with fixed detuning $\Delta$. The fact that gates have varying duration (e.g. a $\pi/2$ rotation has duration half that of a $\pi$ rotation), means that in this implementation errors are gate dependent. Figure 3 shows an example of noise distributions employed in the experiment.

Randomised benchmarking experiments presented in the main text use $\Delta$ sampled from a distribution with $\sigma=1$ kHz, while four fixed detunings are employed in the GST experiments (Fig. 2). Example noise distributions employed in RB are presented in Fig. 3. We note that similar randomised benchmarking results as those shown in the main text have been achieved for several values of $\sigma$. The Rabi frequency is fixed at $\Omega=22.5$ kHz.

| detuning $\Delta$ | $\Delta/\Omega$ |
|---|---|
| 75 Hz | 0.33 % |
| 500 Hz | 2.2 % |
| 1 kHz | 4.4 % |
| 1.4 kHz | 6.2 % |

TABLE I. Engineered detuning cases with fractional errors under Rabi frequency of $\Omega=22.5$ kHz.

In all GST experiments engineered error data was acquired for each sequence, interleaved with the baseline $\Delta=0$ detuning case, such that the datasets are comparable and slow experimental drifts affect them equally. In particular, the cases listed in table I were implemented. For every sequence, all repetitions were taken in direct succession and were not averaged. This approach was employed in order to implement a technique known as "RF blanking" built into the vector signal generator, which allows for superior suppression of both microwave leakage and amplitude instabilities at the edges of pulses. The use of this function, however, comes at the expense of a significant increase in the time overhead associated switching between sequences as an additional sequence must be generated and uploaded to the VSG in order to indicate when RF blanking should be turned on.

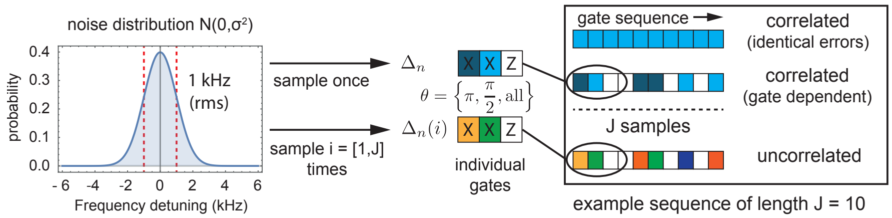


FIG. 2. Each noise realisation is sampled from a distribution specified by its r.m.s. value $\sigma$ either once per sequence (correlated errors) or once per gate, $J$ times per sequences (uncorrelated errors).

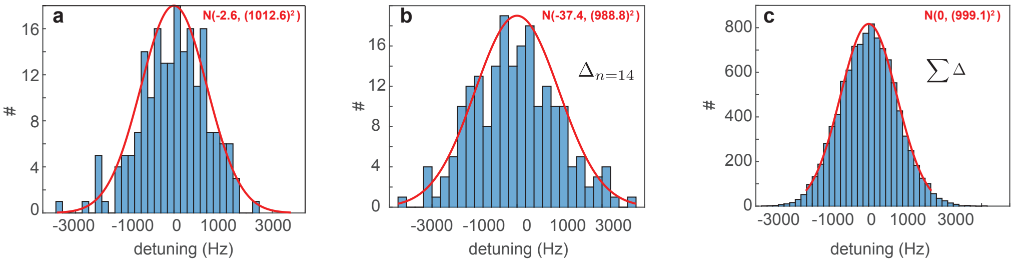


FIG. 3. RB noise distributions for $\sigma = 1$ kHz. **a** 200 noise samples used for correlated noise held constant over complete sequences. **b** Single-gate samples of uncorrelated noise, constituting a single realisation $\Delta_{n=14}$ applied for a $J = 100$ sequence **c** Sum of all 200 uncorrelated noise cases of $J = 100$ samples.

## IV. Linking RB theory to experiment

This section sets out the theory used in this paper to model the RB data presented in the main text. This theory is adapted from the model originally presented Ref. [2], but involves a number of modifications incorporating the previously underappreciated role of the experimental readout process, and the experimental implementation itself (i.e. the structure of the model). We begin by reviewing the original model presented in Ref. [2]. We then describe and physically motivate each of the modifications required to bring this theory into agreement with our experimental data.

In single-qubit RB, random sequences of Clifford operators are implemented. Multiple such randomisations are performed, and from the ensemble statistics of the resulting fidelity measurements, experimentalists may extract the average error per gate (EPG) arising from the system's interaction with the noise environment. For a RB sequence of length $J$, including the final inverting Clifford operation, we write the net operation as the operator product

$$\mathcal{S}_{\boldsymbol{\eta}} \equiv \prod_{j=1}^{J} \mathcal{C}_{\eta_j} \tag{12}$$

where $\mathcal{C}_{\eta_j}$ are Clifford operators (see Table III), $\eta_j$ are random variables sampled uniformly from the set $\{1, 2, ..., 24\}$ indexing all elements of the Clifford group, and the indexing sequence $\boldsymbol{\eta} = (\eta_1, \eta_2, ..., \eta_J)$ describes a distinct RB randomisation. These outcomes are typically constrained by requiring $\mathcal{S}_{\boldsymbol{\eta}} \equiv \hat{\mathbb{I}}$ by choosing $\mathcal{C}^{\dagger}_{\eta_J} = \prod_{j=1}^{J-1} \mathcal{C}_{\eta_j}$, resulting in $24^{J-1}$ distinct possibilities. Under the system's interaction with the underlying noise environment, however, the target Clifford operations $\mathcal{C}_{\eta_j}$ are instead imperfectly implemented as $\tilde{\mathcal{C}}_{\eta_j}$, resulting in the *noise-affected* product

$$\tilde{\mathcal{S}}_{\boldsymbol{\eta},\boldsymbol{\delta}} \equiv \prod_{j=1}^{J} \tilde{\mathcal{C}}_{\eta_j} \neq \hat{\mathbb{I}} \tag{13}$$

where $\boldsymbol{\delta}$ denotes the random noise realisation. The operator product is therefore "steered" away from the identity gate, reducing the operational fidelity of implementing the ideal sequence $\mathcal{S}_{\boldsymbol{\eta}}$.

The analytic noise-averaged fidelity, denoted simply by $\langle \mathcal{F} \rangle$, formally cast in terms of the fidelity metric used in the particular

model, is therefore written

$$\langle \mathcal{F} \rangle = \langle \mathcal{F}(\boldsymbol{\eta}_i, \boldsymbol{\delta}_j) \rangle_{\boldsymbol{\delta}} \tag{14}$$

where $\langle \cdot \rangle_{\boldsymbol{\delta}}$ denotes the expectation value of $\mathcal{F}(\boldsymbol{\eta}_i, \boldsymbol{\delta}_j)$ over the noise random variable, for a given Clifford sequence $\boldsymbol{\eta}_i$, and $i$ and $j$ are indexes for sequences and noise realisations respectively. Consequently our goal is to compare the theoretically calculated probability density function (PDF) calculated for $\langle \mathcal{F} \rangle$ against the distribution of noise-averaged survival probabilities.

In the next section we review the original model presented in Ref. [2]. We then proceed to describe and physically motivate each of the modifications required to bring this theory into agreement with our experimental data.

### A. Original analytic model

Below we outline the key elements of the model treated in Ref. [2], and a full derivation can be found therein. We start with the choice of fidelity metric before moving to the structure of the model (the way errors are implemented), which leads to the characteristic 3D random walk statistics and the resulting PDF for $\langle \mathcal{F} \rangle$. This model employs the *trace fidelity* metric, defined by

$$\mathcal{F}_{\text{trace}}\left(\boldsymbol{\eta}, \boldsymbol{\delta}\right) \equiv \left| \frac{1}{2} \text{Tr}\left( \mathcal{S}_{\boldsymbol{\eta}}^{\dagger} \tilde{\mathcal{S}}_{\boldsymbol{\eta},\boldsymbol{\delta}} \right) \right|^2 = \frac{1}{4} \left| \text{Tr}\left( \tilde{\mathcal{S}}_{\boldsymbol{\eta},\boldsymbol{\delta}} \right) \right|^2 \tag{15}$$

to quantify the fidelity of implementing RB sequence $\boldsymbol{\eta}$ in the presence of noise realisation $\boldsymbol{\delta}$. This operator-based metric captures the overlap between ideal, $\mathcal{S}_{\boldsymbol{\eta}}$, and noise-affected sequences, $\tilde{\mathcal{S}}_{\boldsymbol{\eta},\boldsymbol{\delta}}$, via the Hilbert-Schmidt inner product. The expression for the calculated noise-averaged fidelity therefore takes the form

$$\langle \mathcal{F}_{\text{trace}} \rangle = \frac{1}{4} \left\langle \left| \text{Tr}\left( \tilde{\mathcal{S}}_{\boldsymbol{\eta},\boldsymbol{\delta}} \right) \right|^2 \right\rangle_{\boldsymbol{\delta}}. \tag{16}$$

For noise variables distributed as $\delta \sim \mathcal{N}(0, \sigma^2)$ the assumption of small EPGs translates to the condition that $J\sigma^2 \ll 1$. In this case we approximate the $\tilde{\mathcal{S}}_{\boldsymbol{\eta},\boldsymbol{\delta}}$ as a truncated Taylor expansion in $\delta_j$, yielding

$$\tilde{\mathcal{S}}_{\boldsymbol{\eta},\boldsymbol{\delta}} \approx \prod_{j=1}^{J} \left( \hat{\mathbb{I}} + i\delta_j \hat{\sigma}_z - \frac{\delta_j^2}{2} \hat{\sigma}_z^2 + \ldots \right) \mathcal{C}_{\eta_j}. \tag{17}$$

Retaining only leading order terms with non-vanishing trace, which are all the terms with even powers in $\xi$ because $\text{Tr}\left(\hat{\sigma}_z\right) = 0$ and $\text{Tr}\left(\hat{\mathbb{I}}\right) = 2$ we obtain

$$\tilde{\mathcal{S}}_{\boldsymbol{\eta},\boldsymbol{\delta}} \approx \mathcal{S}_{\boldsymbol{\eta}} + \xi_{1,1}^{(2)} + \ldots \tag{18}$$

where, using group theoretic properties of the Clifford group, we may express

$$\xi_{1,1}^{(2)} = -\sum_{j<k} \delta_j \delta_k \mathbf{P}_j \mathbf{P}_k \tag{19}$$

in terms of random signed Pauli operators $\mathbf{P}_m$. Thus,

$$\mathbf{P}_m = x_m \hat{\sigma}_x + y_m \hat{\sigma}_y + z_m \hat{\sigma}_z \equiv \hat{\boldsymbol{r}}_m \cdot \vec{\boldsymbol{\sigma}} \tag{20}$$

where $x_m, y_m, z_m \in \{0, \pm 1\}$ subject to the constraint $|x_m|^2 + |y_m|^2 + |z_m|^2 = 1$ (only one nonzero coefficient), and we define

$$\hat{\boldsymbol{r}}_m \equiv (x_m,\, y_m,\, z_m), \qquad \|\hat{\boldsymbol{r}}_m\| = 1. \tag{21}$$

That is, the $\hat{\boldsymbol{r}}_m \in \{\pm\hat{\boldsymbol{x}}, \pm\hat{\boldsymbol{y}}, \pm\hat{\boldsymbol{z}}\}$ are unit vector pointing uniformly at random along the principle Cartesian axes, mapping the "direction" of the operators $\mathbf{P}_m$ in the operator space spanned by the Pauli operators. Moving to vector notation and using the cyclic property of Pauli operators inside a trace, we obtain

$$\frac{1}{2} \text{Tr}\left( \mathbf{P}_j \mathbf{P}_k \right) = \hat{\boldsymbol{r}}_j \cdot \hat{\boldsymbol{r}}_k. \tag{22}$$

The use of an interleaved $\hat{\sigma}_z$ error model, where error operators are analytically added between Cliffords, yields the central result

$$\langle \mathcal{F}_{\text{trace}} \rangle \approx 1 - \langle \| \vec{\boldsymbol{R}} \|^2 \rangle, \qquad \vec{\boldsymbol{R}} \equiv \sum_{j=1}^{J} \delta_j \hat{\boldsymbol{r}}_j. \tag{23}$$

From this analysis we obtain the following geometric interpretation. Error accumulation over a $J$-gate Clifford sequence maps to a random walk in a three-dimensional vector-space, with step direction $\hat{\boldsymbol{r}}_m$ representing the action of the error unitaries $\mathbf{P}_m$ in the operator space spanned by the Pauli operators ("Pauli space"). The step length, $\delta_m$, captures the integrated phase between the driving field and qubit during execution of the m$^{\text{th}}$ single gate. Correlations in the noise associated with dephasing or detuning type errors therefore map to correlations in the sequence of step lengths specified by $\boldsymbol{\delta}$. Walks which terminate far from the origin correspond to sequences with large net infidelities while those which end near the origin have small infidelities.

For constant errors we assume all noise random variables $\delta_j \equiv \delta$ are identical over a given sequence $\mathcal{S}_{\boldsymbol{\eta}}$. The PDF for the infidelity therefore corresponds to the distance square of an unbiased 3D walk scaled by $\sigma^2$, and takes the form of the gamma distribution

$$1 - \langle \mathcal{F}_{\text{trace}} \rangle \sim \Gamma\left(\alpha = \frac{3}{2}, \beta = \frac{2}{3} J \sigma^2\right) \tag{24}$$

with shape parameter $\alpha = 3/2$ and scale parameter $\beta = \frac{2}{3} J \sigma^2$.

### B. Modified analytic model

We now describe the modifications to the model in Ref. [2] necessary for good agreement with experimental data. Only results are required to analyse the measurements in this paper are presented here and the full derivation will presented independently in the near future. As above, we start with the choice of fidelity metric before moving onto the structure of the error model. We also introduce some scaling factors associated with our experimental implementation.

#### *1. 2D Random Walk*

Our measurement procedure is described in the main text and first section of this supplement. The critical element in the current discussion revolves around the detection procedure and its relationship to measurable quantities in the theory laid out in [2]. Our experiment involve a projective measurement onto the $z$-axis of the Bloch sphere and therefore corresponds to the quantum mechanical probability defined by

$$\mathcal{F}_{\text{survival}}\left(\boldsymbol{\eta}, \boldsymbol{\delta}\right) \equiv |\left\langle 0 \right| \tilde{\mathcal{S}}_{\boldsymbol{\eta},\boldsymbol{\delta}} \left| 0 \right\rangle|^2 \tag{25}$$

which we refer to as survival probability. This metric is sufficiently different from the *trace* fidelity defined in [2] to prevent good agreement between first-principles PDF calculations described therein and experimental projective measurements. Substituting Eq. 17 into Eq. 25, and reevaluating the leading order terms one can show

$$\langle \mathcal{F}_{\text{survival}} \rangle = 1 - \langle \| \vec{\boldsymbol{R}}_x \|^2 \rangle - \langle \| \vec{\boldsymbol{R}}_y \|^2 \rangle \tag{26}$$

$$= \langle \mathcal{F}_{\text{trace}} \rangle + \langle \| \vec{\boldsymbol{R}}_z \|^2 \rangle \tag{27}$$

where

$$\vec{\boldsymbol{R}}_\alpha = \sum_{j=1}^{J} \delta_j \alpha_j, \qquad \alpha = \{x, y, z\} \tag{28}$$

and $\vec{\boldsymbol{R}}_x + \vec{\boldsymbol{R}}_y + \vec{\boldsymbol{R}}_z = \vec{\boldsymbol{R}}$ in Eq. 23. That is, the walk steps in the $\hat{\sigma}_z$ direction (measurement basis) do not contribute to state infidelity. By projecting the final state $\tilde{\mathcal{S}}_{\boldsymbol{\eta},\boldsymbol{\delta}} \left| 0 \right\rangle$ onto measurement basis ($\hat{\sigma}_z$) we become "blind" to error accumulation along this degree of freedom in Pauli space. By contrast, the trace fidelity involves no such projection, and measures errors associated with all operator outcomes in SU(2). Equation 26 shows that survival probability maps to a $J$-step random walk in $\mathbb{R}^3$ *projected onto a 2D subspace* (*i.e.* the $xy$-plane). This is formally equivalent to a random walk strictly in $\mathbb{R}^2$ of $\frac{2}{3}J$ steps. Once averaged over random noise variable, $\delta$, $\langle \mathcal{F} \rangle$ still follows a gamma distribution with updated shape and scale parameters.

### 2. Concurrent Error Model

The last modification is in the structure of the error model itself. Our error model involves the application of a laboratory detuning between the VSG output and qubit transition which extends during a nonzero-duration driven operation. This is to be contrasted with the use of interleaved Pauli-$\hat{\sigma}_z$ rotations following each gate as in Ref. [2]. Good quantitative agreement with experimental data requires an error model incorporating concurrent dephasing errors using the unitary model described in III; the standard model employed in [2] underestimates the actual error as it does not capture depolarising effects that accumulate under a continuous dephasing field. Current work is undergoing to derive the particular nature of a completely general gamma distribution under these circumstances, however, for our particular gate implementation style (instantaneous $\hat{\sigma}_z$ rotations, identity gates are idle for $\tau_\pi$) and quasi-DC slowly-varying noise we find:

$$1 - \langle \mathcal{F}_{\text{survival}} \rangle \sim \Gamma\left(\alpha = 1, \beta = \frac{2}{3} J\sigma^2 \left(\frac{1}{2} + \frac{\pi^2}{96}\right)\right). \tag{29}$$

In table II also include the expectation and variance for survival probability in the case of quasi-DC miscalibration and rapidly-varying noise. These vary by factors of order unity relative to previous calculations.

| Noise type | $\mathbb{E}(\mathcal{I})$ | $\mathbb{V}(\mathcal{I})$ |
|---|---|---|
| Quasi-DC miscalibration | $\frac{2J\sigma^2}{3}\left(\frac{1}{2} + \frac{\pi^2}{96}\right)$ | $\frac{J^2\sigma^4}{9}\left(\frac{1}{2} + \frac{\pi^2}{96}\right)^2\left(\frac{12}{n} + 2\right)$ |
| Rapidly varying | $\frac{2J\sigma^2}{3}\left(\frac{1}{2} + \frac{\pi^2}{96}\right)$ | $\frac{4J^2\sigma^4}{9}\left(\frac{1}{2} + \frac{\pi^2}{96}\right)^2\left(\frac{1}{n} + \frac{3\times 0.526}{2}\frac{n-1}{n}\frac{1}{J}\right)$ |

TABLE II. Calculation of the first two moments of the noise averaged survival probabilities under concurrently applied noise. These functions are plotted in figures 2b and c.

## V. Clifford Group representation for a single qubit

A unitary operation $\mathcal{C}$ is an element of the *Clifford group* if

$$\mathcal{C}\mathcal{P}\mathcal{C}^\dagger = \mathcal{P} \tag{30}$$

where we have defined the *Pauli group*

$$\mathcal{P} = \{\pm\hat{\mathbb{I}}, \pm\hat{\sigma}_x, \pm\hat{\sigma}_y, \pm\hat{\sigma}_z\}. \tag{31}$$

That is, the Clifford group is the normaliser of the Pauli group, where for every Pauli operation $P \in \mathcal{P}$, there is another $P' \in \mathcal{P}$ such that $\mathcal{C}P\mathcal{C}^\dagger = P'$. For a single qubit, the set of all such $\mathcal{C}$ may be thought of as rotations of the Bloch sphere that permute the orientation of $\pm\hat{\sigma}_x, \pm\hat{\sigma}_y, \pm\hat{\sigma}_z$ in the Cartesian basis associated with the Pauli operators, which we refer to as "Pauli space". To obtain a clearer physical picture of these operations, consider associating $\hat{\sigma}_x$ to any of the six Cartesian axes $\{\pm\hat{\boldsymbol{x}}, \pm\hat{\boldsymbol{y}}, \pm\hat{\boldsymbol{z}}\}$. With this axis fixed, we may rotate the axes about $\hat{\sigma}_x$ into four possible orientations while preserving $xyz$ right-handedness. This is the action of the $\mathcal{C}$ group: the group of rotational symmetries of the cube.

We construct our representation as follows. Let $R_i(\theta)$ represent one of nine elementary unitaries generating a *clockwise* rotation (looking down the axis of rotation toward the origin) through angle $\theta \in \{\pi, \pm\pi/2\}$ about axis $i \in \{x, y, z\}$. The three $\pi$ rotations correspond to

$$R_{x,y,z}(\pi) \equiv \hat{\sigma}_x, \hat{\sigma}_y, \hat{\sigma}_z \tag{32}$$

and we use the shorthand

$$R_i^{\pm} \equiv R_i(\pm\pi/2), \qquad i \in \{x, y, z\} \tag{33}$$

for the remaining six $\pi/2$ rotations. For example, the action of the operators $R_i^{\pm}$ on the Pauli operators/axes is

$$R_x^+ : \quad (\hat{\sigma}_x, \hat{\sigma}_y, \hat{\sigma}_z) \to (\hat{\sigma}_x, -\hat{\sigma}_z, \hat{\sigma}_y) \tag{34}$$

$$R_y^+ : \quad (\hat{\sigma}_x, \hat{\sigma}_y, \hat{\sigma}_z) \to (\hat{\sigma}_z, \hat{\sigma}_y, -\hat{\sigma}_x) \tag{35}$$

$$R_z^+ : \quad (\hat{\sigma}_x, \hat{\sigma}_y, \hat{\sigma}_z) \to (-\hat{\sigma}_y, \hat{\sigma}_x, \hat{\sigma}_z). \tag{36}$$

| # | Gate Name | Action on $(\hat{\sigma}_x, \hat{\sigma}_y, \hat{\sigma}_z)$ | Minimal Sequence(s) | Notes | Gate Time $(\tau_\pi)$ | $\delta_{\text{eff}}$ $(\Delta/\Omega)$ |
|---|---|---|---|---|---|---|
| $\mathcal{C}_1$ | $\hat{\mathbb{I}}$ | $(\hat{\sigma}_x, \hat{\sigma}_y, \hat{\sigma}_z)$ | $R_i^+ R_i^-, \quad i \in \{1,2,3\}$ | Identity | 1 | 1 |
| $\mathcal{C}_2$ | $\hat{\sigma}_x$ | $(\hat{\sigma}_x, -\hat{\sigma}_y, -\hat{\sigma}_z)$ | $\hat{\sigma}_x$ | | 1 | 1 |
| $\mathcal{C}_3$ | $\hat{\sigma}_y$ | $(-\hat{\sigma}_x, \hat{\sigma}_y, -\hat{\sigma}_z)$ | $\hat{\sigma}_y$ | $\pi$ rotation | 1 | 1 |
| $\mathcal{C}_4$ | $\hat{\sigma}_z$ | $(-\hat{\sigma}_x, -\hat{\sigma}_y, \hat{\sigma}_z)$ | $\hat{\sigma}_z$ | | 0 | 0 |
| $\mathcal{C}_5$ | $R_x^+$ | $(\hat{\sigma}_x, -\hat{\sigma}_z, \hat{\sigma}_y)$ | $R_x^+$ | | 1/2 | 1/2 |
| $\mathcal{C}_6$ | $R_y^+$ | $(\hat{\sigma}_z, \hat{\sigma}_y, -\hat{\sigma}_x)$ | $R_y^+$ | $+\pi/2$ rotations | 1/2 | 1/2 |
| $\mathcal{C}_7$ | $R_z^+$ | $(-\hat{\sigma}_y, \hat{\sigma}_x, \hat{\sigma}_z)$ | $R_z^+$ | | 0 | 0 |
| $\mathcal{C}_8$ | $R_x^-$ | $(\hat{\sigma}_x, \hat{\sigma}_z, -\hat{\sigma}_y)$ | $R_x^-$ | | 1/2 | 1/2 |
| $\mathcal{C}_9$ | $R_y^-$ | $(-\hat{\sigma}_z, \hat{\sigma}_y, \hat{\sigma}_x)$ | $R_y^-$ | $-\pi/2$ rotations | 1/2 | 1/2 |
| $\mathcal{C}_{10}$ | $R_z^-$ | $(\hat{\sigma}_y, -\hat{\sigma}_x, \hat{\sigma}_z)$ | $R_z^-$ | | 0 | 0 |
| $\mathcal{C}_{11}$ | | $(-\hat{\sigma}_x, -\hat{\sigma}_z, -\hat{\sigma}_y)$ | $\hat{\sigma}_z R_x^+$ | | 1/2 | 1/2 |
| $\mathcal{C}_{12}$ | | $(-\hat{\sigma}_x, \hat{\sigma}_z, \hat{\sigma}_y)$ | $\hat{\sigma}_z R_x^-$ | | 1/2 | 1/2 |
| $\mathcal{C}_{13}$ | | $(-\hat{\sigma}_y, -\hat{\sigma}_x, -\hat{\sigma}_z)$ | $R_z^+ \hat{\sigma}_x$ | | 1 | 1 |
| $\mathcal{C}_{14}$ | | $(\hat{\sigma}_y, \hat{\sigma}_x, -\hat{\sigma}_z)$ | $R_z^- \hat{\sigma}_x$ | | 1 | 1 |
| $\mathcal{C}_{15}$ | | $(-\hat{\sigma}_y, -\hat{\sigma}_z, \hat{\sigma}_x)$ | $R_z^+ R_x^+$ | | 1/2 | 1/2 |
| $\mathcal{C}_{16}$ | | $(-\hat{\sigma}_y, \hat{\sigma}_z, -\hat{\sigma}_x)$ | $R_z^+ R_x^-$ | | 1/2 | 1/2 |
| $\mathcal{C}_{17}$ | | $(-\hat{\sigma}_z, -\hat{\sigma}_x, \hat{\sigma}_y)$ | $R_x^+ R_z^-$ | | 1/2 | 1/2 |
| $\mathcal{C}_{18}$ | | $(-\hat{\sigma}_z, -\hat{\sigma}_y, -\hat{\sigma}_x)$ | $\hat{\sigma}_z R_y^-$ | | 1/2 | 1/2 |
| $\mathcal{C}_{19}$ | | $(-\hat{\sigma}_z, \hat{\sigma}_x, -\hat{\sigma}_y)$ | $R_z^+ R_y^-$ | | 1/2 | 1/2 |
| $\mathcal{C}_{20}$ | | $(\hat{\sigma}_z, -\hat{\sigma}_x, -\hat{\sigma}_y)$ | $R_z^- R_y^+$ | | 1/2 | 1/2 |
| $\mathcal{C}_{21}$ | $H$ | $(\hat{\sigma}_z, -\hat{\sigma}_y, \hat{\sigma}_x)$ | $\hat{\sigma}_z R_y^+$ | Hadamard | 1/2 | 1/2 |
| $\mathcal{C}_{22}$ | | $(\hat{\sigma}_y, -\hat{\sigma}_z, -\hat{\sigma}_x)$ | $R_z^- R_x^+$ | | 1/2 | 1/2 |
| $\mathcal{C}_{23}$ | | $(\hat{\sigma}_z, \hat{\sigma}_x, \hat{\sigma}_y)$ | $R_z^+ R_y^+$ | | 1/2 | 1/2 |
| $\mathcal{C}_{24}$ | | $(\hat{\sigma}_y, \hat{\sigma}_z, \hat{\sigma}_x)$ | $R_z^- R_x^-$ | | 1/2 | 1/2 |

TABLE III. Representation of the Clifford group for a single qubit from products of elementary rotations. Relevant transformations of the coordinate system $\hat{\sigma}_x, \hat{\sigma}_y, \hat{\sigma}_z$ under the action of each Clifford shown in column 3. Minimal sequence of elementary operations needed to generate each Clifford shown in column 4, in the order of physical gate-application from left to right. Column 5 indicates where these geometric rotations map to logical operations of interest for quantum information. Columns 6 and 7 indicate gate times and effective dephasing strengths incorporating instantaneous, and consequently dephasing-free, $\hat{\sigma}_z$ operations.

Products of these nine elementary operations generate a representation of the 24 elements of the single-qubit Clifford group as tabulated in Table III. We use this prescription to generate numerical simulations verifying our analytic calculations above.

## VI. Limitiations of random walk model

In the main text we suggest that the magnitude of the noise and sequence averaged error in some cases exceeds the validity bounds for the first-order approximations employed in the random-walk framework for RB. While the formal bound in [2] requires $J\sigma^2 \ll 1$, the data presented in figures 2d-g ranges from $J\sigma^2 = 0.05$ to $J\sigma^2 = 0.40$ for 25 gate and 200 gate sequences respectively. Figure 4 shows several simulated survival probability distributions as a function of expectation value $J\sigma^2$. As the value of $J\sigma^2$ increases the shape of the distribution diverges from a gamma distribution with shape parameter 1 (which is mathematically the same as an exponential PDF). Such experimental distributions are in general still well described by gamma distributions if the shape parameter is allowed to vary from 1.

Additionally, we suggest that the scatter of the points in Fig. 3c of the main text partially arises because the $\|\vec{V}\|^2$ is calculated using only the simplified error model that was originally studied in reference [2], where the errors are interleaved throughout the sequence and between gates. To verify this we have performed numerical simulations of sequence survival probabilities under application of the original error model and compare against measured data for the same sequences, but the experimentally relevant concurrent mode(Fig. 5). We observe that the root-mean-squared error between the data points and the best linear fit for the interleaved error case is approximately half that for the concurrently applied error case. However in both cases we still observe a clear linear relationship between walk length and survival probability under the influence of slowly varying noise.

To a first-order approximation we can also incorporate the effects of measurement error (SPAM) by introducing an offset into the gamma distribution describing measured survival probabilities over sequences. We can see this effect using data sets similar to those shown in Fig. 2d-g of the main text, but measured using a detector with higher background counts and analysied with a lower-fidelity detection protocol called “threshold detection".

Threshold detection determines whether each single repetition was in the $|0\rangle$ or $|1\rangle$ state depending on if the detected number

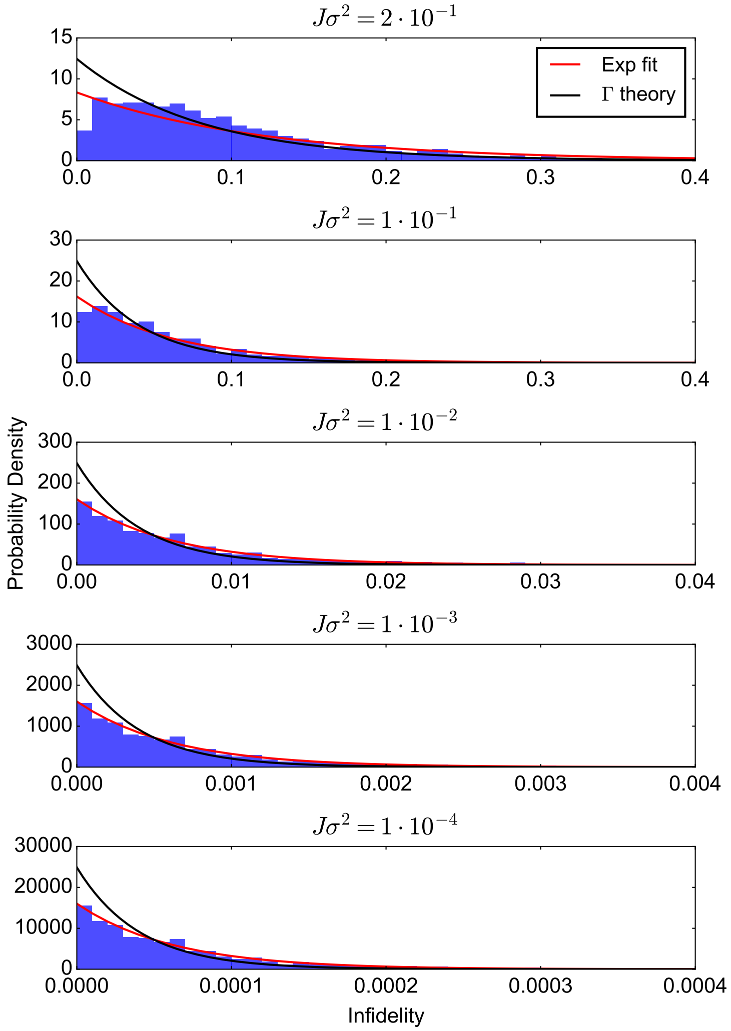


FIG. 4. Survival probability distributions as a function of expectation value $J\sigma^2$. The integral of the simulated histogram values and PDFs are equal to unity. In each case the sequences and noise realisations were kept constant and the magnitude of errors is multiplied by a scalar to produce the correct displayed value of $J\sigma^2$ and the number of gates in a sequence is held constant at $J = 100$. Fits are constrained to maintain shape parameter, $\alpha = 1$, in the gamma distributions.

of photons is above a certain fixed threshold. To find the noise-averaged survival probability we find the mean of all repetitions over noise realisations associated with each sequence. This ultimately leads to a larger measurement error than the method employed in the main text, and permitting quantitative comparisons of the effects. As shown in Fig. 4, the shape parameter diverges from the model if the expectation of the distribution is large, and accordingly we restrict our analysis to data using $J = 10$ to numerically fit an offset for all data sets.

We show such data in figure 6 and overlay the equation 29 with the extracted offset. For comparison we show the same data which is subject to the Bayesian estimation technique described in Sec. I, which is more effective in reducing measurement error. Data remain well described by the gamma distribution with $\alpha = 1$ after incorporation of a fixed offset from unit survival probability.

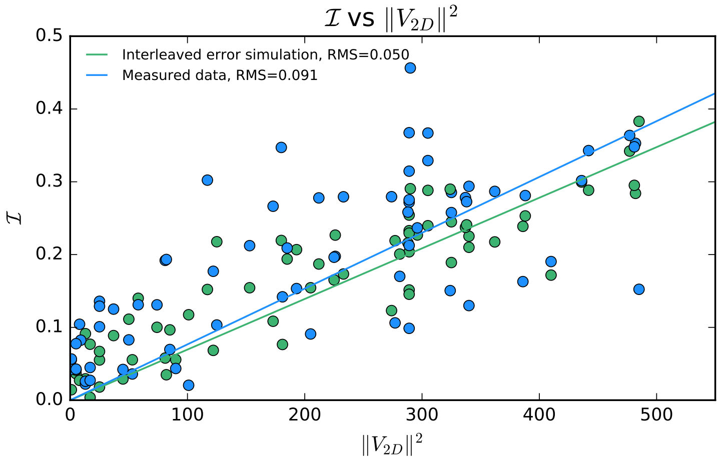


FIG. 5. Noise averaged survival probabilities for measured data subject to concurrently applied noise (blue circles) and simulated outcomes where the interleaved error model matches ref [2] (blue circles) as a function of calculated $\|\vec{V}_{2D}\|^2$. The solid lines represent linear fits to their associated data sets.

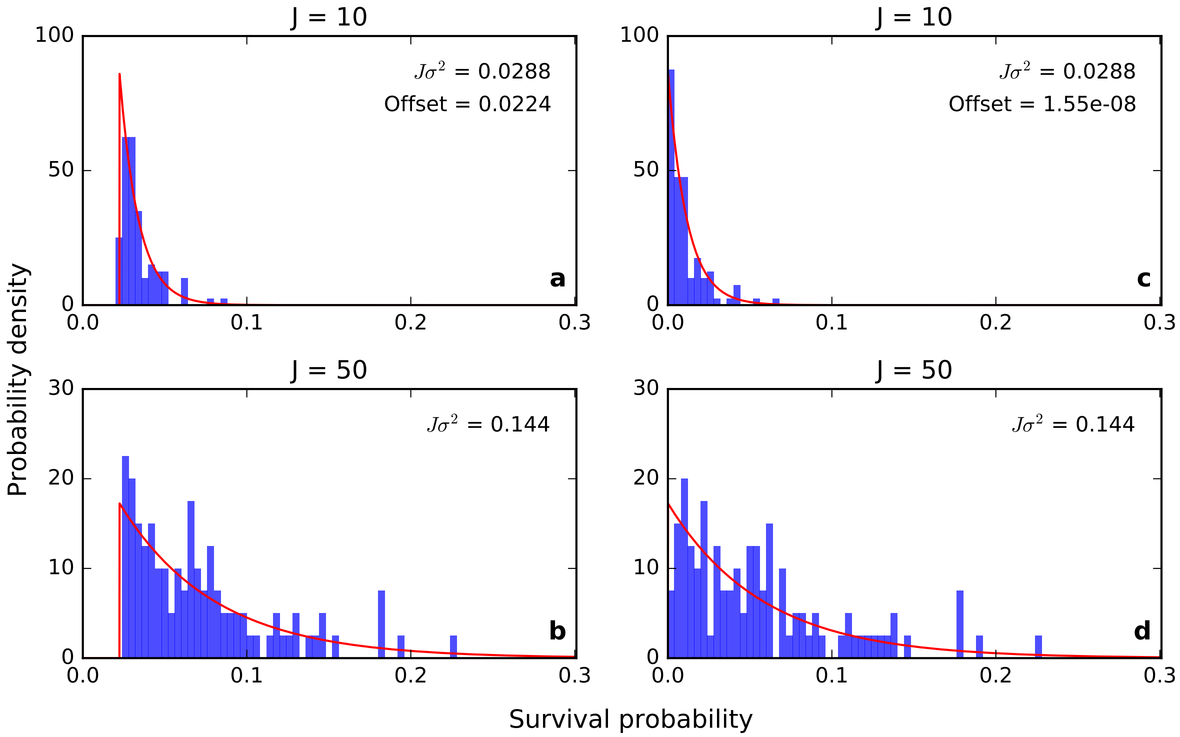


FIG. 6. Survival probabilities distributions of sequences with different numbers of gates with $\sigma^2 = 2.9 \times 10^{-3}$. Figures 6a,b use a simplified analysis technique called "threshold detection" (see text) and figures 6c,d use the bayesian estimation technique outlined in section I. These are overlaid with gamma distributions derived from equation 29 with an additional offset to take into account the level of measurement error in the system calculated from the J=10 data independently for figures 6a,b and 6c,d.

## VII. Randomised Benchmarking baseline data

To quantify our intrinsic background error rate and to ensure that any engineered errors presented in the main text dominate, we perform randomised benchmarking in the absence of any externally applied noise, results shown in Fig. 7. Each sequence was repeated 6000 times and the measurements analysed using the survival probability estimation procedure described above. We find an average error rate of $p_{RB} = 5.99 \times 10^{-5}$ and average state preparation and measurement error of $\kappa = 3.64 \times 10^{-3}$. One clear feature to note is the wide spread of outcomes over sequences which, as mentioned in the main text for the case of engineered noise, may be indicative of gate errors possessing temporal correlations.

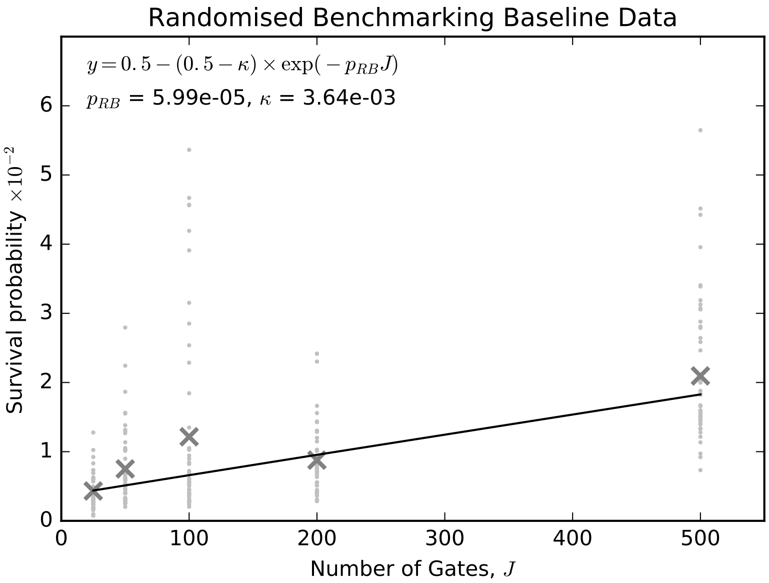


FIG. 7. Randomised banchmarking data in the absence of externally applied noise. individual outcomes for particular sequences are shown as dots and mean of these values as crosses. These mean outcomes for different gate lengths are fit to an exponential equation, shown in panel, weighted by the variance over sequences (black line).

Figure 7 demonstrates a baseline error rate approximately $10^2\times$ lower than the engineered errors typically employed in the main text. We achieve such approximate error rates through use of a phase-stabilised microwave source, and special low-piezoelectric-coefficient coaxial cables providing good amplitude stability. Additionally the low measurement error is due to the large number of repetitions allow the survival probabilities for each sequence to be estimated close to zero. Despite this, one would expect an even lower measurement error given the number of repetitions we implement, but we observe a slightly non-Poissonian photon distribution in the $|1\rangle$ state which is not taken into account in the estimation procedure.

## VIII. GST error simulations

The iPython notebook used to produce the data for Fig. 4 in the main text is included as part of the *Supplementary Material.*

All numerical simulations conducted here have been implemented within the pyGSTi toolkit. We have also independently verified that error models developed in Matlab perform similarly. In addition to the analytic concurrent error models described in the main text we have also compared our findings to a variety of other error models found as in-built options within pyGSTi. The toolkit includes the .rotate() function, corresponding to a post-multiplied error of an amount $\theta$ around the x,y or z axis of the Bloch sphere. It is also possible to simulate the effect of depolarizing noise using pyGSTi built-in functionality. In Fig. 8 below we are using both to investigate the effect of gauge freedom under a variety of error models and using both gatessets.

The extended gate set associated with integration of negative rotations, $\{G_x, G_y, G_i\} \rightarrow \{G_x, G_y, G_i, -G_x, -G_y\}$, also involves extension of the set of germs from the original 11 listed in the methods section to the following enlarged list of 39 entries, where Gxm and Gym stand for the negative rotations:
('Gx',), ('Gy',), ('Gi',), ('Gxm',), ('Gym',),
('Gx', 'Gy',), ('Gxm', 'Gym',), ('Gxm', 'Gy',), ('Gx', 'Gym',),
('Gx', 'Gy', 'Gi',), ('Gx', 'Gi', 'Gy',), ('Gx', 'Gi', 'Gi',), ('Gy', 'Gi', 'Gi',),

('Gxm', 'Gy', 'Gi',), ('Gx', 'Gym', 'Gi',), ('Gxm', 'Gi', 'Gy',), ('Gx', 'Gi', 'Gym',),
('Gxm', 'Gym', 'Gi',), ('Gxm', 'Gi', 'Gym',), ('Gxm', 'Gi', 'Gi',), ('Gym', 'Gi', 'Gi',),
('Gx', 'Gx', 'Gi', 'Gy',), ('Gx', 'Gy', 'Gy', 'Gi',), ('Gxm', 'Gxm', 'Gi', 'Gy',), ('Gxm', 'Gx', 'Gi', 'Gym',),
('Gx', 'Gxm', 'Gi', 'Gym',),('Gx', 'Gx', 'Gi', 'Gym',),('Gx', 'Gxm', 'Gi', 'Gy',),('Gxm', 'Gx', 'Gi', 'Gy',),
('Gxm', 'Gym', 'Gy', 'Gi',), ('Gxm', 'Gy', 'Gym', 'Gi',), ('Gx', 'Gym', 'Gym', 'Gi',),
('Gxm', 'Gy', 'Gy', 'Gi',), ('Gx', 'Gy', 'Gym', 'Gi',), ('Gx', 'Gym', 'Gy', 'Gi',),
('Gxm', 'Gxm', 'Gi', 'Gym',), ('Gxm', 'Gym', 'Gym', 'Gi',),
('Gx', 'Gx', 'Gy', 'Gx', 'Gy', 'Gy',), ('Gxm', 'Gxm', 'Gym', 'Gxm', 'Gym', 'Gym',)

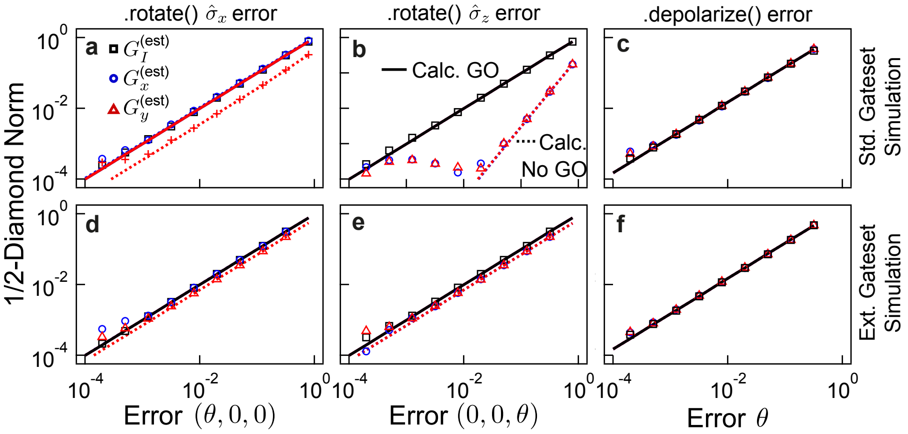


FIG. 8. Comparison of the sensitivity of the standard $\{G_x, G_y, G_i\}$ gate set and an extended version$\{G_x, G_y, G_i, -G_x, -G_y\}$ using the built-in .rotate() and .depolarize function.

## IX. GST experiments and results

In this section we provide a summary of the key results reported by the pyGSTi analysis toolkit [3], version 0.9.2. We show the raw estimates and selected derived quantities from the reports generated by the toolkit and refer to its included tutorials for further descriptions and explanations of the reported quantities. We also provide the datasets, python analysis notebooks and generated reports as separate supplementary files. In these other quantities such as process matrices and the visualized likelihood analyses linked to model violations can be found.

All error cases were measured in direct succession, i.e. for every prescribed GST sequence, $r = 220$ repetitions were recorded for each detuning before proceeding to the next GST sequence. In this way, long term drifts are common mode to all of the separate datasets. The Rabi frequency during all experiments was $\Omega = 22.5$ kHz.

Additional engineered noise cases not considered in detail in the main text are also presented following these tables in a final Section.

TABLE IV. GST estimate of SPAM probabilities

| | $\Delta = 0$ | $\Delta = 75$ Hz | $\Delta = 500$ Hz | $\Delta = 1$ kHz | $\Delta = 1.4$ kHz |
|---|---|---|---|---|---|
| $E$ | 0.0044 $\pm$0.0007 | 0.0043 $\pm$0.0007 | 0.0061 $\pm$0.0008 | 0.0064 $\pm$0.0008 | 0.0069 $\pm$0.0009 |
| $E_c$ | 0.9956 $\pm$0.0033 | 0.9967 $\pm$0.001 | 0.995 $\pm$0.0008 | 0.9943 $\pm$0.0007 | 0.992 $\pm$0.0008 |

Target rotation angles are $\{G_i, G_x, G_y\} = \{0, 0.5, 0.5\}$. Process infidelity, trace distance and diamond norm are ideally 0.

TABLE V. baseline (no detuning error)

| Gate | Rotation Angle | Process Infidelity | $1/2$ Trace Distance | $1/2$ $\diamond$-Norm |
|---|---|---|---|---|
| Gi | $(0.0022 \pm 0.0001)\pi$ | $0.0012 \pm 0.0001$ | $0.0048 \pm 0.0002$ | $0.0048 \pm 0.0002$ |
| Gx | $(0.4995 \pm 0.0001)\pi$ | $0.0001 \pm 0.0001$ | $0.0011 \pm 0.0001$ | $0.0011 \pm 0.0001$ |
| Gy | $(0.4998 \pm 0.0001)\pi$ | $0.0004 \pm 0.0001$ | $0.0009 \pm 0.0001$ | $0.0009 \pm 0.0002$ |

TABLE VI. $\Delta = 75$ Hz detuning error

| Gate | Rotation Angle | Process Infidelity | $1/2$ Trace Distance | $1/2$ $\diamond$-Norm |
|---|---|---|---|---|
| Gi | $(0.0032 \pm 0.0001)\pi$ | $0.0012 \pm 0.0001$ | $0.0059 \pm 0.0002$ | $0.006 \pm 0.0002$ |
| Gx | $(0.4996 \pm 0.0001)\pi$ | $0.0001 \pm 0.0001$ | $0.0011 \pm 0.0001$ | $0.0011 \pm 0.0001$ |
| Gy | $(0.5001 \pm 0.0001)\pi$ | $0.0004 \pm 0.0001$ | $0.0009 \pm 0.0002$ | $0.0011 \pm 0.0002$ |

TABLE VII. $\Delta = 500$ Hz detuning error

| Gate | Rotation Angle | Process Infidelity | $1/2$ Trace Distance | $1/2$ $\diamond$-Norm |
|---|---|---|---|---|
| Gi | $(0.0119 \pm 4 \times 10^{-5})\pi$ | $0.0002 \pm 0.0001$ | $0.019 \pm 0.0002$ | $0.0191 \pm 0.0002$ |
| Gx | $(0.4999 \pm 0.0001)\pi$ | $0.0003 \pm 0.0001$ | $0.0011 \pm 0.0001$ | $0.0012 \pm 0.0001$ |
| Gy | $(0.5007 \pm 0.0001)\pi$ | $0.0003 \pm 0.0001$ | $0.0016 \pm 0.0001$ | $0.0018 \pm 0.0002$ |

TABLE VIII. $\Delta = 1000$ Hz detuning error

| Gate | Rotation Angle | Process Infidelity | $1/2$ Trace Distance | $1/2$ $\diamond$-Norm |
|---|---|---|---|---|
| Gi | $(0.0236 \pm 5 \times 10^{-5})\pi$ | $0.0014 \pm 0.0001$ | $0.0371 \pm 0.0001$ | $0.0372 \pm 0.0001$ |
| Gx | $(0.5009 \pm 0.0001)\pi$ | $0.0002 \pm 0.0001$ | $0.0022 \pm 0.0001$ | $0.0022 \pm 0.0002$ |
| Gy | $(0.5013 \pm 5 \times 10^{-5})\pi$ | $0.0001 \pm 0.0001$ | $0.0027 \pm 0.0001$ | $0.0028 \pm 0.0002$ |

TABLE IX. $\Delta = 1400$ Hz detuning error

| Gate | Rotation Angle | Process Infidelity | $1/2$ Trace Distance | $1/2$ $\diamond$-Norm |
|---|---|---|---|---|
| Gi | $(0.033 \pm 4 \times 10^{-5})\pi$ | $0.0027 \pm 0.0001$ | $0.052 \pm 0.0003$ | $0.052 \pm 0.0003$ |
| Gx | $(0.5016 \pm 0.0001)\pi$ | $-5 \times 10^{-6} \pm 0.0001$ | $0.0035 \pm 0.0001$ | $0.0035 \pm 0.0002$ |
| Gy | $(0.5016 \pm 5 \times 10^{-5})\pi$ | $0.0002 \pm 0.0001$ | $0.0036 \pm 0.0001$ | $0.0036 \pm 0.0001$ |

TABLE X. The GST estimate of the logic gate operations under in the absence of any additive detuning error ($\Delta = 0$ Hz).

| Gate | Superoperator (Pauli basis) | 95% C.I. $1/2$-width |
|---|---|---|
| Gi | $\begin{pmatrix} 1 & 0.0001 & -0.0001 & 1 \times 10^{-5} \\ 0.0002 & 1 & 0.0005 & -0.0055 \\ -0.0001 & 0.0009 & 1 & 0.0052 \\ -0.0001 & 0.0047 & -0.0046 & 0.9954 \end{pmatrix}$ | $\begin{pmatrix} 0.0001 & 0.0001 & 0.0001 & 0.0001 \\ 0.0001 & 0.0001 & 0.0002 & 0.0003 \\ 0.0002 & 0.0002 & 0.0001 & 0.0003 \\ 0.0003 & 0.0003 & 0.0003 & 0.0003 \end{pmatrix}$ |
| Gx | $\begin{pmatrix} 1 & 1 \times 10^{-5} & -0.0002 & 0.0002 \\ 0.0001 & 1 & 0.0007 & 0.001 \\ 4 \times 10^{-5} & 0.0004 & 0.0018 & -0.9998 \\ 0.0001 & -0.0007 & 0.9998 & 0.0011 \end{pmatrix}$ | $\begin{pmatrix} 0.0001 & 0.0001 & 0.0001 & 0.0001 \\ 0.0002 & 0.0001 & 0.0003 & 0.0003 \\ 0.0002 & 0.0003 & 0.0003 & 0.0001 \\ 0.0001 & 0.0003 & 0.0001 & 0.0003 \end{pmatrix}$ |
| Gy | $\begin{pmatrix} 1 & 0.0002 & -0.0001 & 0.0002 \\ 0.0002 & 0.0004 & 0.0012 & 0.9991 \\ -0.0002 & 0.0009 & 1 & -0.0002 \\ -0.0002 & -0.9991 & 0.0005 & 0.0007 \end{pmatrix}$ | $\begin{pmatrix} 0.0001 & 0.0001 & 0.0001 & 0.0001 \\ 0.0002 & 0.0004 & 0.0003 & 0.0001 \\ 0.0002 & 0.0003 & 0.0001 & 0.0003 \\ 0.0002 & 0.0001 & 0.0003 & 0.0004 \end{pmatrix}$ |

TABLE XI. The GST estimate of the logic gate operations under $\Delta = 75$ Hz detuning error.

| Gate | Superoperator (Pauli basis) | 95% C.I. $1/2$-width |
|---|---|---|
| Gi | $\begin{pmatrix} 1 & -2 \times 10^{-5} & -3 \times 10^{-5} & 2 \times 10^{-5} \\ -1 \times 10^{-5} & 0.9999 & 0.0055 & -0.0067 \\ -0.0001 & -0.0041 & 0.9998 & 0.0058 \\ 0.0001 & 0.0065 & -0.0068 & 0.9956 \end{pmatrix}$ | $\begin{pmatrix} 0.0001 & 0.0001 & 0.0001 & 0.0001 \\ 0.0002 & 0.0001 & 0.0003 & 0.0005 \\ 0.0002 & 0.0002 & 0.0001 & 0.0003 \\ 0.0003 & 0.0004 & 0.0004 & 0.0003 \end{pmatrix}$ |
| Gx | $\begin{pmatrix} 1 & 5 \times 10^{-5} & -0.0002 & 0.0002 \\ 0.0002 & 1 & 0.0007 & 0.0012 \\ 0.0001 & 0.0001 & 0.0018 & -0.9998 \\ 0.0001 & -0.0007 & 0.9998 & 0.0007 \end{pmatrix}$ | $\begin{pmatrix} 0.0001 & 0.0001 & 0.0001 & 0.0001 \\ 0.0002 & 0.0001 & 0.0003 & 0.0003 \\ 0.0001 & 0.0003 & 0.0003 & 0.0001 \\ 0.0001 & 0.0003 & 0.0001 & 0.0003 \end{pmatrix}$ |
| Gy | $\begin{pmatrix} 1 & 0.0002 & -0.0001 & 0.0002 \\ 0.0003 & -0.0006 & 0.0015 & 0.9993 \\ -0.0001 & 0.0009 & 1 & 0.0002 \\ -0.0003 & -0.9993 & 0.0004 & -2 \times 10^{-6} \end{pmatrix}$ | $\begin{pmatrix} 0.0001 & 0.0001 & 0.0001 & 0.0001 \\ 0.0001 & 0.0004 & 0.0003 & 0.0001 \\ 0.0002 & 0.0003 & 0.0001 & 0.0003 \\ 0.0001 & 0.0001 & 0.0003 & 0.0004 \end{pmatrix}$ |

TABLE XII. The GST estimate of the logic gate operations under $\Delta = 500$ Hz detuning error.

| Gate | Superoperator (Pauli basis) | 95% C.I. ½-width |
|---|---|---|
| Gi | $\begin{pmatrix} 1 & -5\times10^{-5} & -0.0001 & 0.0001 \\ -0.0001 & 0.9993 & 0.0357 & -0.0097 \\ -0.0001 & -0.0347 & 0.9994 & 0.0083 \\ 0.0001 & 0.0092 & -0.0088 & 1.0004 \end{pmatrix}$ | $\begin{pmatrix} 0.0001 & 0.0001 & 0.0001 & 0.0001 \\ 0.0002 & 0.0001 & 0.0003 & 0.0004 \\ 0.0002 & 0.0003 & 0.0001 & 0.0004 \\ 0.0002 & 0.0004 & 0.0004 & 0.0001 \end{pmatrix}$ |
| Gx | $\begin{pmatrix} 1 & 0.0001 & -0.0002 & 0.0002 \\ 0.0002 & 1 & 0.0011 & 0.0018 \\ 3\times10^{-5} & 0.0005 & 0.0003 & -0.9995 \\ 0.0001 & -0.0012 & 0.9994 & 3\times10^{-5} \end{pmatrix}$ | $\begin{pmatrix} 0.0001 & 0.0001 & 0.0001 & 0.0001 \\ 0.0002 & 0.0001 & 0.0003 & 0.0003 \\ 0.0001 & 0.0003 & 0.0003 & 0.0001 \\ 0.0001 & 0.0003 & 0.0001 & 0.0003 \end{pmatrix}$ |
| Gy | $\begin{pmatrix} 1 & 0.0002 & -0.0001 & 0.0002 \\ 0.0002 & -0.0026 & 0.0016 & 0.9994 \\ -0.0002 & 0.0011 & 1 & -0.0007 \\ -0.0002 & -0.9995 & 0.0012 & -0.0018 \end{pmatrix}$ | $\begin{pmatrix} 0.0001 & 0.0001 & 0.0001 & 0.0001 \\ 0.0001 & 0.0003 & 0.0003 & 0.0001 \\ 0.0002 & 0.0003 & 0.0001 & 0.0003 \\ 0.0001 & 0.0001 & 0.0003 & 0.0003 \end{pmatrix}$ |

TABLE XIII. The GST estimate of the logic gate operations under $\Delta = 1$ kHz detuning error.

| Gate | Superoperator (Pauli basis) | 95% C.I. ½-width |
|---|---|---|
| Gi | $\begin{pmatrix} 1 & 4\times10^{-5} & -0.0001 & 3\times10^{-6} \\ -1\times10^{-5} & 0.9973 & 0.0732 & -0.0073 \\ -0.0002 & -0.0731 & 0.9972 & 0.0078 \\ 0.0001 & 0.0093 & -0.009 & 1 \end{pmatrix}$ | $\begin{pmatrix} 0.0001 & 0.0001 & 0.0001 & 0.0001 \\ 0.0003 & 0.0001 & 0.0005 & 0.0005 \\ 0.0002 & 0.0005 & 0.0001 & 0.0005 \\ 0.0002 & 0.0005 & 0.0005 & 0.0001 \end{pmatrix}$ |
| Gx | $\begin{pmatrix} 1 & 4\times10^{-5} & -0.0002 & 0.0002 \\ 0.0001 & 0.9999 & 0.0017 & 0.0023 \\ -2\times10^{-5} & 0.0014 & -0.0026 & -0.9997 \\ -1\times10^{-5} & -0.0021 & 0.9997 & -0.003 \end{pmatrix}$ | $\begin{pmatrix} 0.0001 & 0.0001 & 0.0001 & 0.0001 \\ 0.0002 & 0.0001 & 0.0003 & 0.0003 \\ 0.0001 & 0.0003 & 0.0003 & 0.0001 \\ 0.0001 & 0.0003 & 0.0001 & 0.0003 \end{pmatrix}$ |
| Gy | $\begin{pmatrix} 1 & 0.0002 & -0.0001 & 0.0002 \\ 0.0002 & -0.0045 & 0.0022 & 0.9998 \\ -0.0002 & 0.0019 & 1 & -0.0015 \\ -0.0001 & -0.9998 & 0.0018 & -0.0037 \end{pmatrix}$ | $\begin{pmatrix} 0.0001 & 0.0001 & 0.0001 & 0.0001 \\ 0.0001 & 0.0002 & 0.0003 & 0.0001 \\ 0.0002 & 0.0003 & 0.0001 & 0.0003 \\ 0.0001 & 0.0001 & 0.0003 & 0.0002 \end{pmatrix}$ |

TABLE XIV. The GST estimate of the logic gate operations under $\Delta = 1.4$ kHz detuning error.

| Gate | Superoperator (Pauli basis) | 95% C.I. ½-width |
|---|---|---|
| Gi | $\begin{pmatrix} 1 & 0.0001 & -4\times10^{-5} & -4\times10^{-5} \\ 0.0001 & 0.9947 & 0.1035 & -0.0045 \\ -0.0001 & -0.1032 & 0.9946 & 0.005 \\ 0.0001 & 0.0053 & -0.0054 & 1 \end{pmatrix}$ | $\begin{pmatrix} 0.0001 & 0.0001 & 0.0001 & 0.0001 \\ 0.0003 & 0.0001 & 0.0006 & 0.0005 \\ 0.0003 & 0.0006 & 0.0001 & 0.0005 \\ 0.0002 & 0.0006 & 0.0005 & 0.0001 \end{pmatrix}$ |
| Gx | $\begin{pmatrix} 1 & 0.0001 & -0.0002 & 0.0002 \\ 0.0002 & 1 & 0.0035 & 0.0031 \\ 0.0001 & 0.0031 & -0.0051 & -1.0001 \\ 3\times10^{-5} & -0.0027 & 1 & -0.0047 \end{pmatrix}$ | $\begin{pmatrix} 0.0001 & 0.0001 & 5\times10^{-5} & 0.0001 \\ 0.0002 & 0.0001 & 0.0003 & 0.0002 \\ 0.0001 & 0.0002 & 0.0003 & 0.0001 \\ 0.0001 & 0.0003 & 0.0001 & 0.0003 \end{pmatrix}$ |
| Gy | $\begin{pmatrix} 1 & 0.0002 & -0.0001 & 0.0002 \\ 0.0002 & -0.005 & 0.0031 & 0.9995 \\ -0.0003 & 0.0027 & 0.9999 & -0.0031 \\ -0.0002 & -0.9996 & 0.0035 & -0.0052 \end{pmatrix}$ | $\begin{pmatrix} 0.0001 & 0.0001 & 0.0001 & 5\times10^{-5} \\ 0.0001 & 0.0002 & 0.0003 & 0.0001 \\ 0.0002 & 0.0003 & 0.0001 & 0.0003 \\ 0.0001 & 0.0001 & 0.0003 & 0.0002 \end{pmatrix}$ |

The tables below report the comparison between computed estimate based on GST's CPTP model and the experimental data given to the analysis routine. Here, $N_S$ and $N_p$ are the number of gate strings and fit parameters, respectively. The quantity $2\Delta\log(\mathcal{L})$ measures the goodness of fit of the GST model (small is better) and is expected to lie within $[k-\sqrt{2k}, k+\sqrt{2k}]$ where $k = N_s - N_p$. $N_\sigma = (2\Delta\log(\mathcal{L}) - k)/\sqrt{2k}$ is the number of standard deviations from the mean and provides an indication of the agreement with the CPTP model underlying the GST analysis. The star rating is a crude indication of the strength of model violation seen. Detailed reports and data are available on request. More detailed explanations can be found in the tutorials and generated reports of the pyGSTi toolkit [3].

TABLE XV. baseline (no detuning error)

| L | $2\Delta\log(\mathcal{L})$ | $k$ | $2\Delta\log(\mathcal{L}) - k$ | $\sqrt{2k}$ | $N_\sigma$ | $N_s$ | $N_p$ | Rating |
|---|---|---|---|---|---|---|---|---|
| 1 | 49.457 | 52 | -2.5432 | 10.198 | -0.25 | 92 | 40 | ★★★★★ |
| 2 | 119.78 | 128 | -8.2157 | 16 | -0.51 | 168 | 40 | ★★★★★ |
| 4 | 456.12 | 401 | 55.122 | 28.32 | 1.95 | 441 | 40 | ★★★★ |
| 8 | 860.83 | 777 | 83.827 | 39.421 | 2.13 | 817 | 40 | ★★★★ |
| 16 | 1368.5 | 1161 | 207.46 | 48.187 | 4.31 | 1201 | 40 | ★★★★ |
| 32 | 1922.7 | 1545 | 377.69 | 55.588 | 6.79 | 1585 | 40 | ★★★★ |
| 64 | 3082.7 | 1929 | 1153.7 | 62.113 | 18.6 | 1969 | 40 | ★★★★ |
| 128 | 7860 | 2313 | 5547 | 68.015 | 81.6 | 2353 | 40 | ★★★ |
| 256 | $2\times10^4$ | 2697 | $2\times10^4$ | 73.444 | $2\times10^2$ | 2737 | 40 | ★★ |

TABLE XVI. 75 Hz detuning

| L | $2\Delta\log(\mathcal{L})$ | $k$ | $2\Delta\log(\mathcal{L}) - k$ | $\sqrt{2k}$ | $N_\sigma$ | $N_s$ | $N_p$ | Rating |
|---|---|---|---|---|---|---|---|---|
| 1 | 59.185 | 52 | 7.1851 | 10.198 | 0.7 | 92 | 40 | ★★★★★ |
| 2 | 145.12 | 128 | 17.117 | 16 | 1.07 | 168 | 40 | ★★★★ |
| 4 | 448.75 | 401 | 47.751 | 28.32 | 1.69 | 441 | 40 | ★★★★ |
| 8 | 889.84 | 777 | 112.84 | 39.421 | 2.86 | 817 | 40 | ★★★★ |
| 16 | 1358 | 1161 | 197.02 | 48.187 | 4.09 | 1201 | 40 | ★★★★ |
| 32 | 1882.3 | 1545 | 337.29 | 55.588 | 6.07 | 1585 | 40 | ★★★★ |
| 64 | 2903.9 | 1929 | 974.94 | 62.113 | 15.7 | 1969 | 40 | ★★★★ |
| 128 | 7715.9 | 2313 | 5402.9 | 68.015 | 79.4 | 2353 | 40 | ★★★ |
| 256 | $2\times10^4$ | 2697 | $2\times10^4$ | 73.444 | $2\times10^2$ | 2737 | 40 | ★★ |

TABLE XVII. 500 Hz detuning

| L | $2\Delta\log(\mathcal{L})$ | $k$ | $2\Delta\log(\mathcal{L}) - k$ | $\sqrt{2k}$ | $N_\sigma$ | $N_s$ | $N_p$ | Rating |
|---|---|---|---|---|---|---|---|---|
| 1 | 67.508 | 52 | 15.508 | 10.198 | 1.52 | 92 | 40 | ★★★★ |
| 2 | 138.08 | 128 | 10.082 | 16 | 0.63 | 168 | 40 | ★★★★★ |
| 4 | 424.26 | 401 | 23.261 | 28.32 | 0.82 | 441 | 40 | ★★★★★ |
| 8 | 882.46 | 777 | 105.46 | 39.421 | 2.68 | 817 | 40 | ★★★★ |
| 16 | 1329.8 | 1161 | 168.78 | 48.187 | 3.5 | 1201 | 40 | ★★★★ |
| 32 | 1857.7 | 1545 | 312.67 | 55.588 | 5.62 | 1585 | 40 | ★★★★ |
| 64 | 2861.8 | 1929 | 932.76 | 62.113 | 15 | 1969 | 40 | ★★★★ |
| 128 | 5637 | 2313 | 3324 | 68.015 | 48.9 | 2353 | 40 | ★★★★ |
| 256 | $1\times10^4$ | 2697 | 7957.3 | 73.444 | $1\times10^2$ | 2737 | 40 | ★★★ |

TABLE XVIII. 1 kHz detuning

| L | $2\Delta\log(\mathcal{L})$ | $k$ | $2\Delta\log(\mathcal{L})-k$ | $\sqrt{2k}$ | $N_\sigma$ | $N_s$ | $N_p$ | Rating |
|---|---|---|---|---|---|---|---|---|
| 1 | 55.22 | 52 | 3.2203 | 10.198 | 0.32 | 92 | 40 | ★★★★★ |
| 2 | 129.21 | 128 | 1.2101 | 16 | 0.08 | 168 | 40 | ★★★★★ |
| 4 | 426.82 | 401 | 25.821 | 28.32 | 0.91 | 441 | 40 | ★★★★★ |
| 8 | 774.03 | 777 | -2.9656 | 39.421 | -0.08 | 817 | 40 | ★★★★★ |
| 16 | 1308.9 | 1161 | 147.9 | 48.187 | 3.07 | 1201 | 40 | ★★★★ |
| 32 | 1862.4 | 1545 | 317.37 | 55.588 | 5.71 | 1585 | 40 | ★★★★ |
| 64 | 2565.1 | 1929 | 636.14 | 62.113 | 10.2 | 1969 | 40 | ★★★★ |
| 128 | 4743.6 | 2313 | 2430.6 | 68.015 | 35.7 | 2353 | 40 | ★★★★ |
| 256 | 7622.6 | 2697 | 4925.6 | 73.444 | 67.1 | 2737 | 40 | ★★★★ |

TABLE XIX. 1.4 kHz detuning

| L | $2\Delta\log(\mathcal{L})$ | $k$ | $2\Delta\log(\mathcal{L})-k$ | $\sqrt{2k}$ | $N_\sigma$ | $N_s$ | $N_p$ | Rating |
|---|---|---|---|---|---|---|---|---|
| 1 | 80.609 | 52 | 28.609 | 10.198 | 2.81 | 92 | 40 | ★★★★ |
| 2 | 149.36 | 128 | 21.356 | 16 | 1.33 | 168 | 40 | ★★★★ |
| 4 | 447.87 | 401 | 46.871 | 28.32 | 1.66 | 441 | 40 | ★★★★ |
| 8 | 897.86 | 777 | 120.86 | 39.421 | 3.07 | 817 | 40 | ★★★★ |
| 16 | 1427.1 | 1161 | 266.15 | 48.187 | 5.52 | 1201 | 40 | ★★★★ |
| 32 | 1970 | 1545 | 425.04 | 55.588 | 7.65 | 1585 | 40 | ★★★★ |
| 64 | 2585.6 | 1929 | 656.62 | 62.113 | 10.6 | 1969 | 40 | ★★★★ |
| 128 | 4421.8 | 2313 | 2108.8 | 68.015 | 31 | 2353 | 40 | ★★★★ |
| 256 | 7240.9 | 2697 | 4543.9 | 73.444 | 61.9 | 2737 | 40 | ★★★★ |

### X. Overview of GST experimental datasets for various error models

Here we summarise additional engineered noise cases studied in the course of our experiments. References are provided to the pyGSTi outputs which are included as supplemental files.

The evaluation of all datasets used pyGSTi version 0.9.2 available at http://www.pygsti.info and the corresponding reports are included. The slow drift cases were evaluated using version 0.9.3, which includes a summary page of the complete system environment (python packaged used etc.).

All experiments were implemented using a Rabi frequency of $\Omega = 22.5$ kHz as baseline. Every sequence and case was repeated 220 times before proceeding. In the data post processing (see *Supplemental Material*) some of these repetitions were rejected due to obvious technical errors such as ion loss or cooling failure leading to slightly different numbers of total counts throughout all sequences.

#### Frequency detuning of the control (maximally correlated error)

For each GST sequence (out of the 2737), we step through 5 cases of a deliberately introduced detuning error and record their results separately:

TABLE XX. cases DC frequency detuning

| Case | relative error ($\Delta/\Omega$) | filename |
|---|---|---|
| baseline/reference | 0 | `baseline.txt` |
| 75 Hz | 0.3% | `DC75Hz.txt` |
| 500 Hz | 2.2% | `DC500Hz.txt` |
| 1 kHz | 4.4% | `DC1kHz.txt` |
| $-1$ kHz | 4.4% | `DC-1kHz.txt` |
| 1.4 kHz | 6.2% | `DC1p4kHz.txt` |

#### Markovian noise (uncorrelated error)

A white noise generator samples a distribution with 500 Hz rms at various speeds (bandwidth). This leads to errors that range from being (on average) constant over a gate duration to varying during a gate. All gates ($\pi/2$) are executed on a time scale of 11 $\mu$s ($\sim$ 91 kHz).

TABLE XXI. cases fast fluctuations

| Case, detuning | bandwidth | filename |
|---|---|---|
| baseline / no detuning | 0 | `baseline2.txt` |
| 500 Hz r.m.s. | 100 Hz | `500Hz_rms_BW_100_Hz.txt` |
| 500 Hz r.m.s. | 1 kHz | `500Hz_rms_BW_1_kHz.txt` |
| 500 Hz r.m.s. | 10 kHz | `500Hz_rms_BW_10_kHz.txt` |
| 500 Hz r.m.s. | 1 MHz | `500Hz_rms_BW_1_MHz.txt` |

#### SPAM

The effect of state preparation and measurement is investigated by deliberately diminishing the initial $|0\rangle$ state fidelity. `Filename: bad_pumping.txt`

#### Miscalibration of microwave amplitude (over-rotation)

We deliberately change increase the Rabi frequency (microwave peak voltage) by 1%, leading to an over-rotation error. `Filename: AM_offset_1pct.txt`

#### Line noise 50 Hz

A very common error source is the oscillation of the qubit transition frequency induced by external magnetic fields emanating from technical sources like power supplies, synchronous with the AC line frequency. We simulate the effect by a deliberate sinusoidal modulation of the microwave frequency using an external signal generator set to 50 Hz. The detuning was varied by (a) $\pm 5$ Hz and (b) $\pm 20$ Hz. These applied oscillations add to intrinsic line noise that, at the 3.2 Gauss operating point of our

hyperfine qubit, is estimated to be on the order of 2 Hz, corresponding to 1 mG field variations.
`Filenames: 50HzFM_5Hz.txt, 50HzFM_20Hz.txt`

**Slow drifts**

We are simulating the effect of common slow drifts in laboratory environments, e.g. a slowly oscillating HVAC system.

**frequency drift**
This effect could be caused by a power supply driving magnetic field coils, leading to a slow (36 min period) $\pm 25$ Hz variation in the detuning induced by quantization field drifts. `Filename: slow_AM_drift_1pct.txt`

**amplitude drift**
This effect could be caused by gain variations in a microwave amplifier, leading to a slow (36 min period) $\pm 1\%$ variation in the Rabi frequency. `Filename: slowFM25Hz.txt`

---

[1] Wölk, S., Piltz, C., Sriarunothai, T. & Wunderlich, C. State selective detection of hyperfine qubits. *Journal of Physics B: Atomic, Molecular and Optical Physics* **48**, 075101 (2015).
[2] Ball, H., Stace, T. M., Flammia, S. T. & Biercuk, M. J. Effect of noise correlations on randomized benchmarking. *Physical Review A* **93**, 022303 (2016). URL `http://link.aps.org/doi/10.1103/PhysRevA.93.022303`.
[3] Nielsen, E., Rudinger, K., Gamble, J. K. & Blume-Kohout, R. pygsti: A python implementation of gate set tomography. available at http://github.com/pygstio (2016).
